# Supplementary material for: Network constraints on learnability of probabilistic motor sequences
Source: arXiv:1709.03000 ancillary file (2018-10-30)
Supplement: Supplementary file 1 [file network_constraints_graph_learning_supplement.pdf]

# Network constraints on learnability of probabilistic motor sequences

**Ari E. Kahn**[1,2,3], **Elisabeth A. Karuza**[4], **Jean M. Vettel**[3,5,2], **and Danielle S. Bassett**[2,6,7,8,9]

[1]Department of Neuroscience, University of Pennsylvania, Philadelphia, PA 19104 USA

[2]Department of Bioengineering, University of Pennsylvania, Philadelphia, PA 19104 USA

[3]Human Research and Engineering Directorate, U.S. Army Research Laboratory, Aberdeen, MD 21001 USA

[4]Department of Psychology, University of Pennsylvania, Philadelphia, PA 19104 USA

[5]Department of Psychological and Brain Sciences, University of California, Santa Barbara, CA 93106 USA

[6]Department of Electrical & Systems Engineering, University of Pennsylvania, Philadelphia, PA 19104 USA

[7]Department of Neurology, Perelman School of Medicine, University of Pennsylvania, Philadelphia, PA 19104 USA

[8]Department of Physics & Astronomy, College of Arts and Sciences, University of Pennsylvania, Philadelphia, PA 19104 USA

[9]To whom correspondence should be addressed: dsb@seas.upenn.edu.

## Contents


1 Supplementary Methods 2

2 Supplementary Figures 7

3 Supplementary Tables 12


# 1 Supplementary Methods

### Overview of Experimental Design

We ran three experiments, each consisting of two back-to-back *stages* that differed in which graph and walk type was used to generate the stimulus sequence (Supplementary Table 1). The first experiment used either a *modular*, *lattice*, or *random* graph to generate a sequence of 1500 stimuli via a random walk on the graph. The second stage of the experiment used a fully connected graph to generate a sequence of 500 stimuli via a random walk on the graph (amounting to a random stimulus order.) The second experiment consisted of 1500 trials of a random walk on a modular graph, followed by 500 trials of a Hamiltonian walk on the same graph, allowing us to confirm that learned differences transferred to a different walk type on the same graph structure. The first stage of the third experiment consisted of a sequence of 1500 stimuli via a random walk on either a modular graph, a lattice graph, or a random graph. However, unlike the first experiment, the second stage was another sequence of 1500 stimuli via a random walk on one of the remaining two sparse structured graph types.

### Reaction Time Comparison Between Experiments

We plotted the average RT per 10 trials across the entire experiment, comparing experiment type, to confirm consistency of our data across experiments (Supplementary Fig. 1). We find that learners showed very similar trajectories for the first stage, replicated across the three experiments. We likewise observe similar performance for Experiments 2 and 3 in the second stage for the next 500 trials. Experiment 3 also demonstrates a plateau in improvement for the trials 2000-3000, not evident in Experiments 1 and 2 due to their shorter lengths. Note that due to walks derived from the fully connected graph introducing less predictable transitions, as well as additional novel edges to learn, stage 2 of Experiment 1 shows a noticeably larger mean RT than the other two experiments.

### Reaction Time Comparison Between Graph Types

We additionally plotted differences in RT by graph type across the entire experiment, pooling data from all three experiments (Supplementary Fig. 2). We observe significantly more variability between graph types in stage 2, which may reflect inherent differences that are not evident while learners are still adapting to the biomechanics of the task. Also note that there is significantly more data for each individual graph type in stage 1. We find the differences in stage 2 of interest, but given the large between-subject variance in performance, we have solely based our analyses differences in RT between graph type on within-subject measures.

### Persistence of Surprisal Effect

In the main manuscript, we showed that the magnitude of the surprisal effect on a random walk in stage 1 was a strong predictor of persistence of the surprisal effect on those same edges when the walk was switched to a Hamiltonian walk in stage 2. Specifically, we found that a subject's coefficient for cross-cluster surprisal in the random walk was a significant predictor of that same subject's coefficient for the cross-cluster surprisal in the Hamiltonian walk (Fig. 2D; $t(57) = 10.089, p < 0.001$, Pearson's correlation coefficient $r = 0.8$, 95% confidence interval: 0.69 to 0.88). We note that one uninteresting possible explanation for this effect is that it could be driven by the assignment of faster or slower motor actions to the post-transition nodes for certain subjects, thereby leading to timing differences associated with those nodes that carry over into the second stage of the experiment. To ensure that such a potential explanation was not relevant to our study, we performed a permutation test in which we randomly reassigned labels indicating which nodes in the graph we considered to be 'cross-cluster edges'.

In performing this permutation test, we wished to maintain constraints that existed in the baseline modular graph. Thus, in performing the 1000 permutations, no two edges chosen as 'cross-cluster edges' within the same permutation could share a node with each other, but were otherwise selected at random. In the permuted data, we again estimated the correlation between the surprisal effect in stage 1 and the surprisal effect in stage 2, and we compared the distribution of observed correlation values to the true value observed on the modular graph (Supplementary Fig. 3). We found that out of 1000 permutations, only 20 led to surprisal effect correlations greater than or equal to that observed under the true assignment, strongly supporting the notion that this persistence effect is reliant on the underlying cross-cluster surprisal effect and is not an artifact of motor action assignment.

### Node Statistics on Random Graphs

To quantify the impact of node-level statistics that could explain RT differences within a single graph, we examined several traditional graph metrics, including degree, clustering coefficient, node betweenness centrality, and edge betweenness centrality

(see Analytical Approach in the main manuscript for definitions). One significant confound for the random graph was that its varied topology might lead to certain nodes being much more highly visited than other nodes, and thus certain nodes might display differing RTs merely because the node had been visited more frequently. In contrast, we were more interested in how less trivial aspects of the node's topological role might influence RT, so we regressed out the number of times a node had been visited. We reported two statistics in the main text, node betweenness centrality and node degree, which were significantly related to performance both before and after regressing out the number of times visited. Here we report full results (both pre- and post- regressing out times visited) for node degree (Supplementary Fig. 4), node betweenness centrality (Supplementary Fig. 5), edge betweenness centrality (Supplementary Fig. 6), and node clustering coefficient (Supplementary Fig. 7). For all four figures, we plotted the average RT for each node/edge ($z$-scored within each subject) against the node/edge statistic. The left panel displays results obtained when not regressing out times a node/edge was visited, and the right panel displays results obtained after regressing out times a node/edge was visited. Due to non-normality in node statistic distributions, we tested correlations using Kendall's $\tau$. We find that all three node statistics show a significant correlation with RT once times a node is visited is regressed out (node betweenness centrality: $\tau = 0.044, n = 2655, p < 0.001$, node degree: $\tau = 0.072, n = 2655, p < 0.001$, node clustering coefficient: $\tau = 0.034, n = 2655, p = 0.014$), but not edge betweenness centrality ($\tau = 0.002, n = 5310, p = 0.87$). Only node degree and node betweenness centrality are also significant without regressing out times visited (node betweenness centrality: $\tau = -0.045, n = 2655, p < 0.001$, node degree: $\tau = -0.045, n = 2655, p = 0.001$, node clustering coefficient: $\tau = 0.007, n = 2655, p = 0.61$, edge betweenness centrality: $\tau = 0.002, n = 5310, p = 0.87$). Intriguingly, the direction of the relationship for node degree and node betweenness centrality and RT reverses once the number of times visited is regressed out, suggesting both a significant impact of degree and betweenness centrality on how often a learner is exposed to a given node, leading to lower predicted RTs with increased exposure, but also an increased RT when times visited is accounted for, suggesting that a more central role in the network makes a node harder to predict.

## Differences Between Targets

We examined whether different finger actions exhibited reliable differences in reaction time. We subdivided the subjects from experiments one and three into three groups, based on which of the three graphs (modular, random, or lattice) they had seen in the first stage of either experiment, and averaged the per-target reaction times within each group. We plotted the reaction times and found that the relative ordering was remarkably similar between the three subject groups, spanning a range of nearly 500ms between the slowest and fastest targets (Supplementary Fig. 8).

### Nonlinear Effect of Trial

By fitting a simple mixed effects model $RT \sim Trial * Stage + (1 + Trial * Stage \mid Subject)$ to data from experiments one and three, we observed a significant effect of trial (linear mixed effects model, $t(108) = 12.34, p < 0.001, SE = 12.141$). However, by visual inspection it is clear that the relation between reaction time and trial is not linear. We compared modeling of RT *versus* trial number as a linear fit *versus* as RT *versus* log(trial) (Supplementary Fig. 9). We found that log(trial) provided a substantially better fit, as represented by the AIC of $RT \sim Trial * Stage + (1 + Trial * Stage|\text{Subject})$ versus $RT \sim \log(Trial) * Stage + (1 + \log(Trial) * Stage \mid Subject)$: linear fit AIC = 2981849, log fit AIC = 2980365, df = 15). In the remaining analyses in this study, we therefore fit all models to log(trial).

### Effect of Addition of Edges on Surprisal Effect

Here we ask whether the cross-cluster surprisal effect persisted for a motor response when the topological role of that response within the network was altered. To address this question, we analyzed data acquired from the traversal of the modular graph in Experiment 1. In stage 1, we labeled edges as transition edges if their adjoining nodes were in distinct clusters. In stage 2 when a fully connected graph was used, we kept the labels from stage 1 indicating if an edge had previously served as a transition edge. We ignored all trials on edges not present in stage 1, with the goal of eliminating any RT increase associated with the traversal of a novel edge. We then plotted the average RT as a function of trial number for both stage 1 and stage 2, separating the trials according to whether they were transition edges *versus* non-transition edges (Supplementary Fig. 10).

We observed consistently higher RTs on transition edges than on non-transition edges in stage 1, representative of the surprisal effect. We also observed higher RTs in stage 2 for (previous) transition edges than (previous) non-transition edges, though the effect was smaller in magnitude. We quantified these observations by fitting a mixed-effects model to stage 2 data for Experiment 1: $RT \sim Target + Trial * (Transition\ in\ 1 + Edge\ in\ 1) + (1 + Trial * (Transition\ in\ 1 + Edge\ in\ 1) \mid \text{Subject})$. Here '*Transition in 1*' marks whether an edge corresponded to a prior transition edge, bridging two clusters in stage 1; similarly, '*Edge in 1*' marks whether that edge had been present in stage 1 at all. We found a significant effect for Transition Type, with an expected increase of 113.71 ms (linear mixed effects model, $t(30) = 2.1, p = 0.044$, $SE = 54.23$, 95% confidence interval: 7.43 to 219.99; Supplementary Table 6). This effect confirms that a significant difference in RT remains for transition *versus* non-transition edges even after the addition of novel edges to the graph. Paired with our other findings that the surprisal effect persists when the graph traversal is modified, this result strongly suggests that the role of these edges between clusters of stimuli uniquely positions them within the learning process, as they continue to incur different processing costs even in scenarios such

as a Hamiltonian walk or a fully connected graph where we would not expect such a difference to emerge on its own.

To verify that this effect was not driven by outlier timepoints, we refit the same model after removing all trials whose RT was more than 3 SDs away from the mean for that subject and transition type. The significant relationship between RT and Transition Type persisted, with an expected increase of 132.33 ms (linear mixed effects model, $t(29.6) = 2.5, p = 0.019$, $SE = 29.63$, 95% confidence interval: 74.26 to 190.40). These results indicate that the effect is not explained by outlier timepoints.

## 2 Supplementary Figures

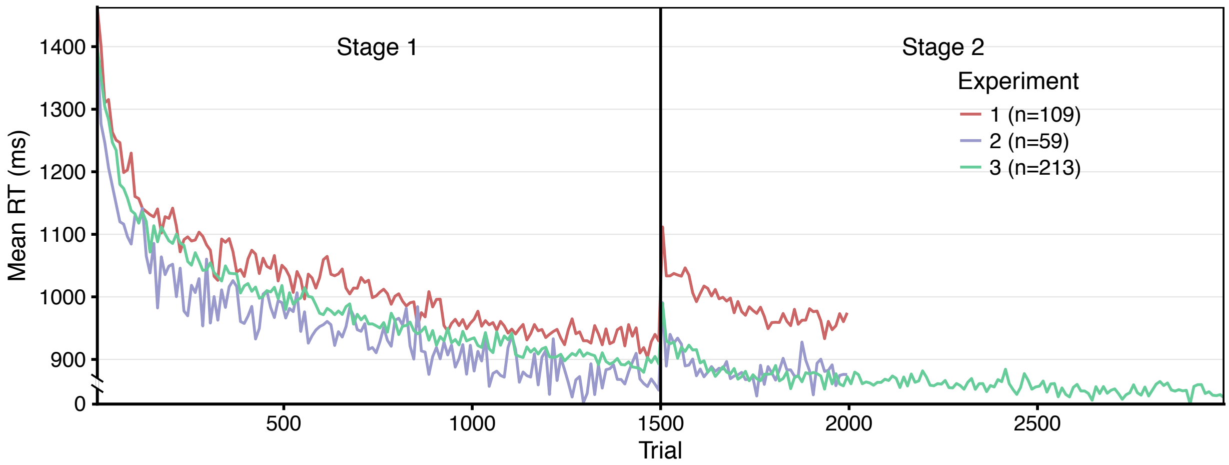


**Supplementary Figure 1. Reaction Time Comparison Between Experiments.** Mean RT per 10 trials, across trials for all three experiments. The three lines correspond to the three experiments. The left half (trials 1-1500) corresponds to trials in stage 1, and the right half (trials 1501-3000) corresponds to trials in stage 2. Experiments 1 and 3 only consisted of 500 trials for stage 2.

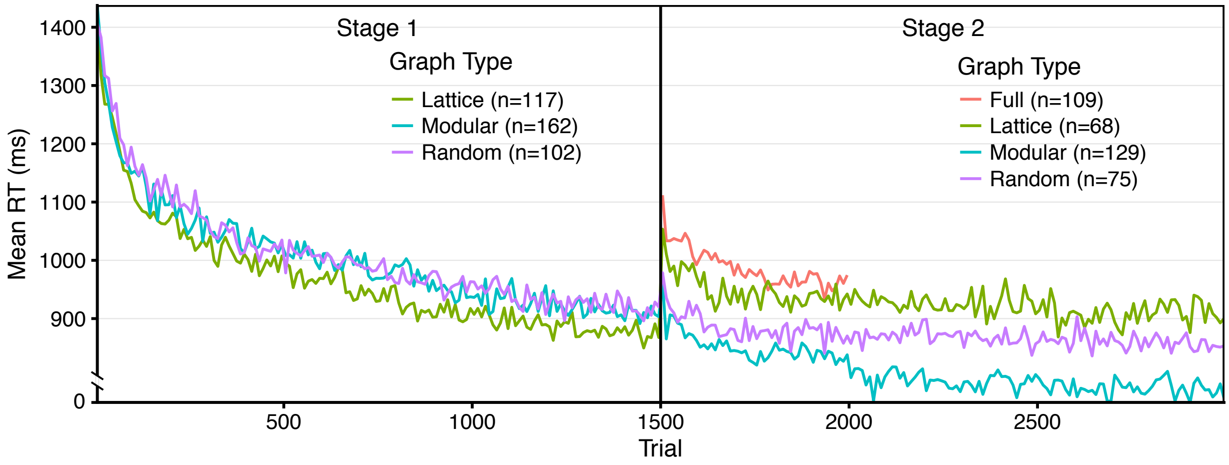


**Supplementary Figure 2. Reaction Time Comparison Between Graph Types.** Mean RT per 10 trials, across trials for all graph types used to generate walks. The left half (trials 1-1500) corresponds to trials in stage 1, and the right half (trials 1501-3000) corresponds to trials in stage 2. As the Fully Connected graph only occurred in experiment 1, there is no data for trials 1-1500, or trials 2001-3000.

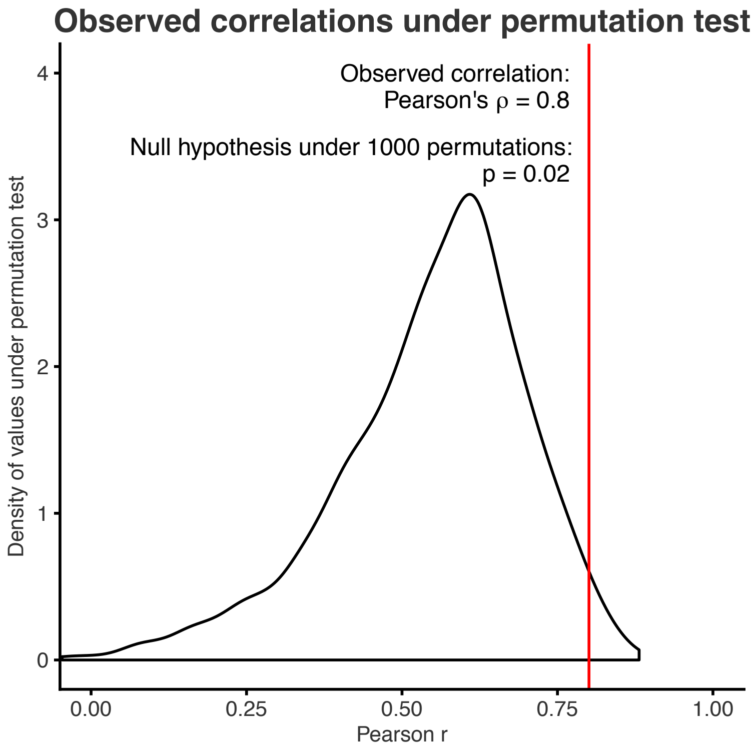


**Supplementary Figure 3. Permutation Test for the Persistence of the Surprisal Effect.** We performed a permutation test (1000 permutations) where we reassigned which graph edges are labeled as 'cross-cluster' edges. We then recalculated the correlation between the surprisal effect in stage 1 and the surprisal effect in stage 2 across all 59 subjects. We found that only 20 of the 1000 permutations led to a correlation value greater than or equal to that originally observed. This result verifies that the observed persistence of the surprisal effect was not due to individual idiosyncrasies in how subjects responded to the motor actions assigned to the nodes comprising the cross-cluster edges.

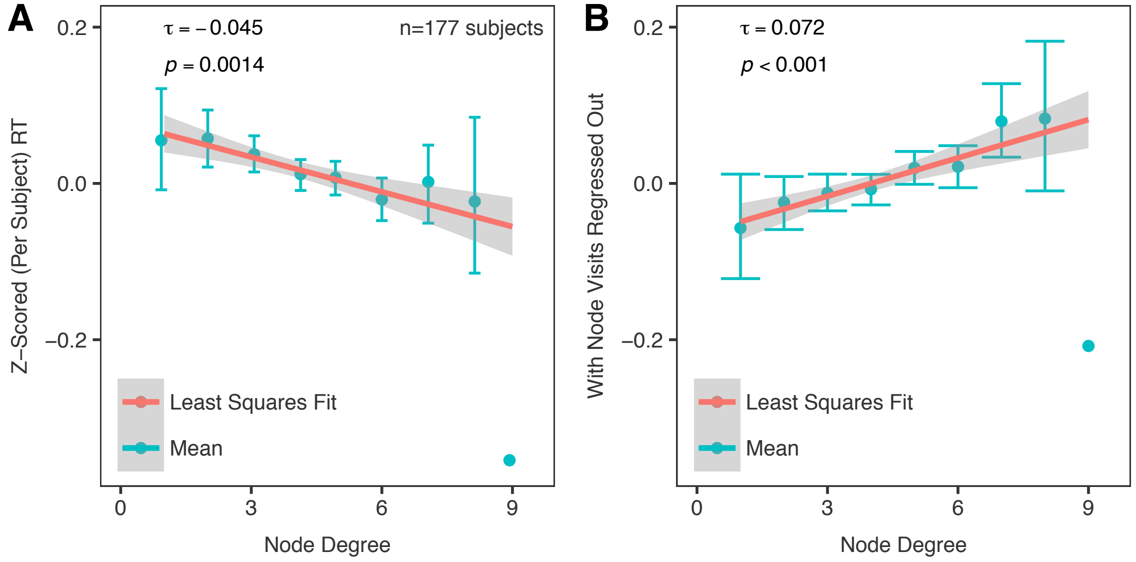


**Supplementary Figure 4. Relation Between Node Degree and Reaction Time.** *(A)* Relationship between node degree and reaction time (RT). The red regression line shows the least squares fit with a gray 95% confidence envelope. Reported correlation is based on Kendall's $\tau$. *(B)* The same relationship is plotted, however, the total times a node has been visited has been regressed out from RTs. Data from n=177 subjects.

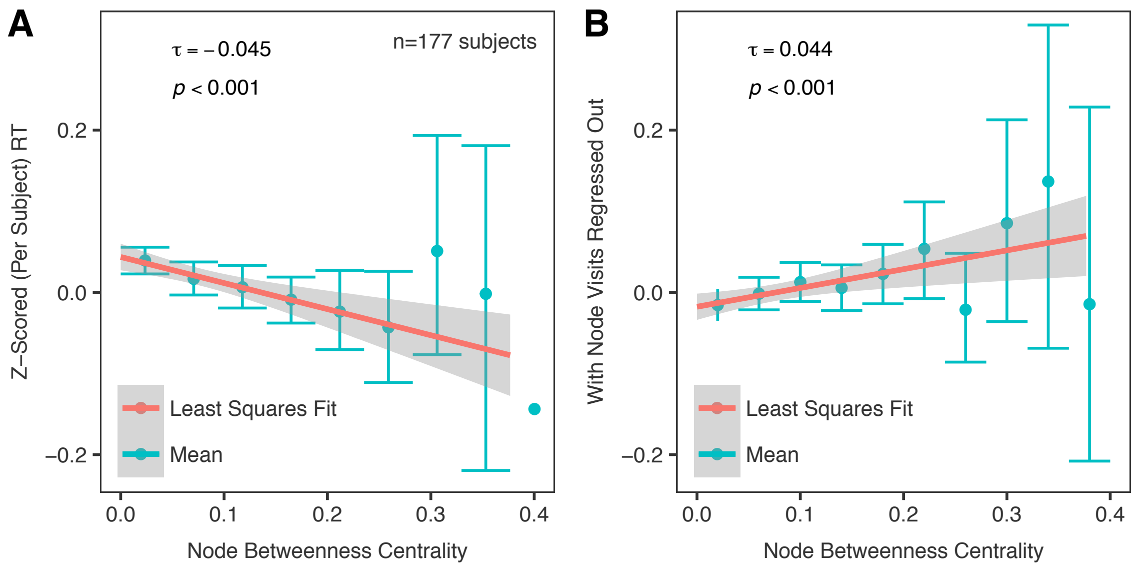


**Supplementary Figure 5. Relation Between Node Betweenness Centrality and Reaction Time.** *(A)* Relationship between node betweenness centrality and reaction time (RT). The red regression line shows the least squares fit with a gray 95% confidence envelope. Reported correlation is based on Kendall's $\tau$. *(B)* The same relationship is plotted, however, the total times a node has been visited has been regressed out from RTs. Data from n=177 subjects.

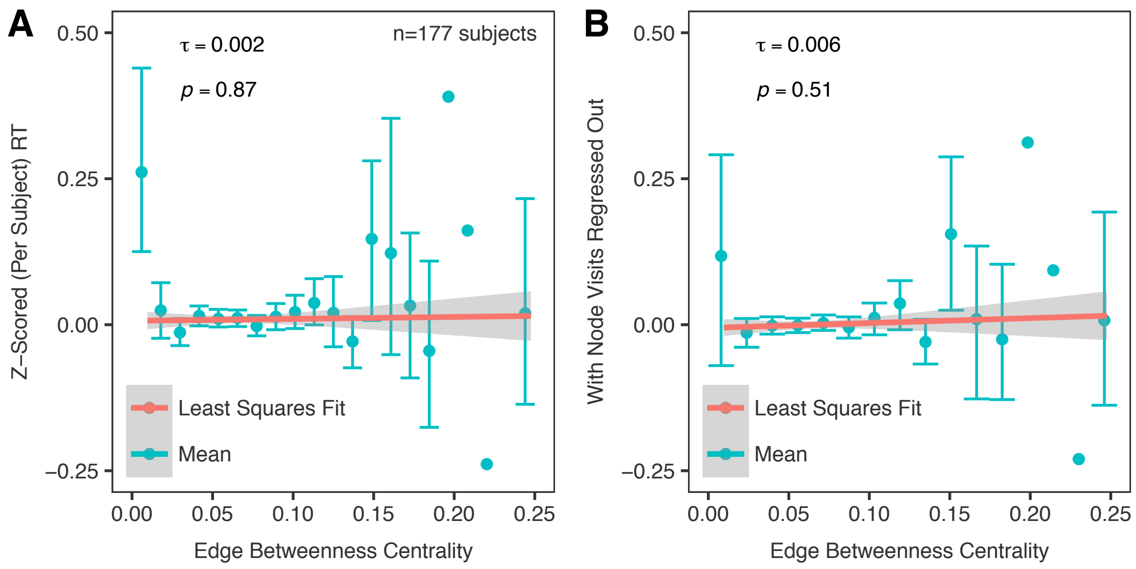


**Supplementary Figure 6. Relation Between Edge betweenness Centrality and Reaction Time.** *(A)* Relationship between edge betweenness centrality and reaction time (RT). The red regression line shows the least squares fit with a gray 95% confidence envelope. Reported correlation is based on Kendall's $\tau$. *(B)* The same relationship is plotted, however, the total times a node has been visited has been regressed out from RTs. Data from n=177 subjects.

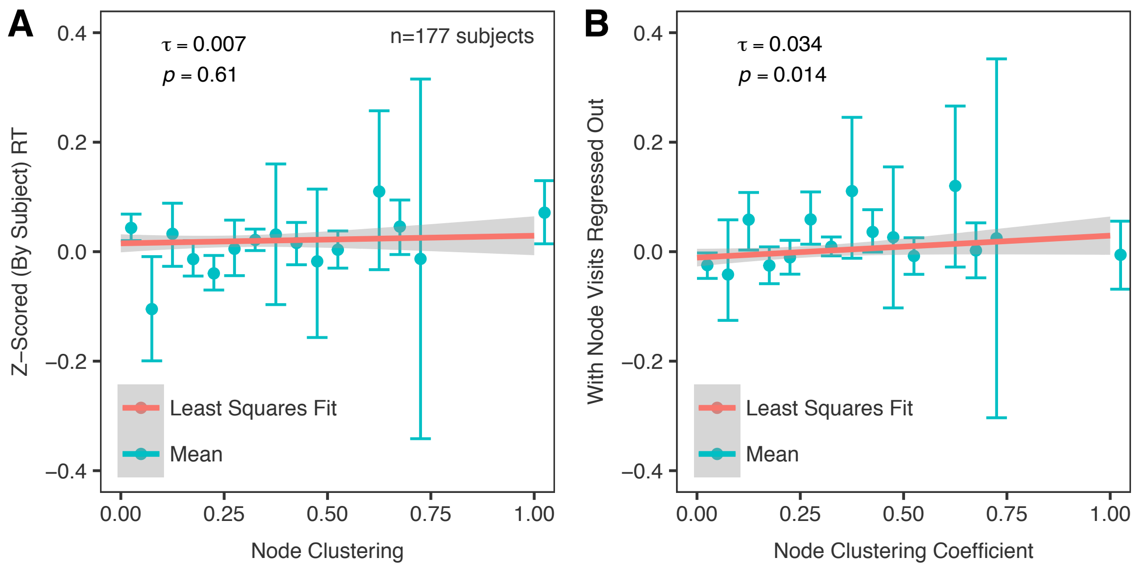


**Supplementary Figure 7. Relation Between Node Clustering Coefficient and Reaction Time.** *(A)* Relationship between node clustering coefficient and reaction time (RT). The red regression line shows the least squares fit with a gray 95% confidence envelope. Reported correlation is based on Kendall's $\tau$. *(B)* The same relationship is plotted, however, the total times a node has been visited has been regressed out from RTs. Data from n=177 subjects.

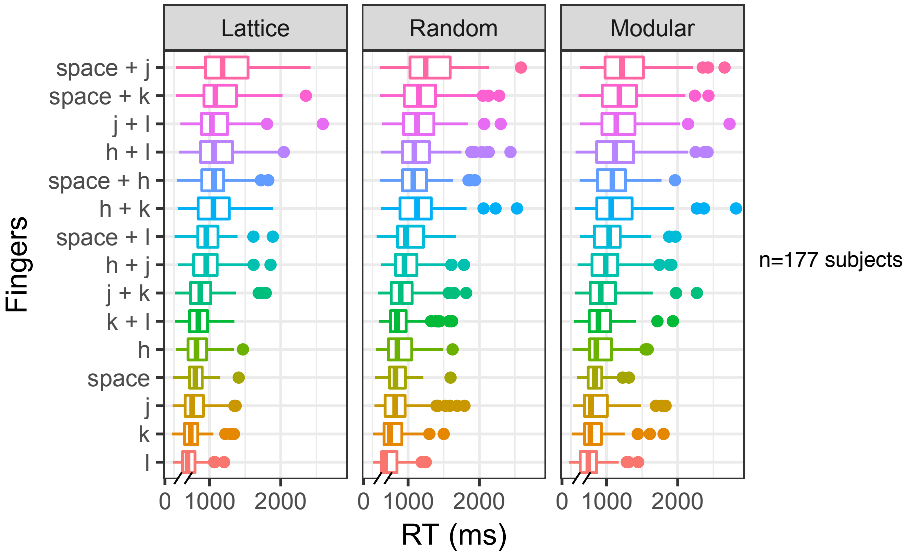


**Supplementary Figure 8. Target Reaction Time Across Subject Groups.** We plotted the average reaction time (RT) for each target, based on the keys required, across three separate groups of subjects, divided based on graph type. Each of the three columns is a separate group of subjects from the first stage of either experiment. Each box indicates median and quartiles. We find a remarkably consistent biomechanical RT difference associated with each target. Respectively, n=117, n=102, and n=103.

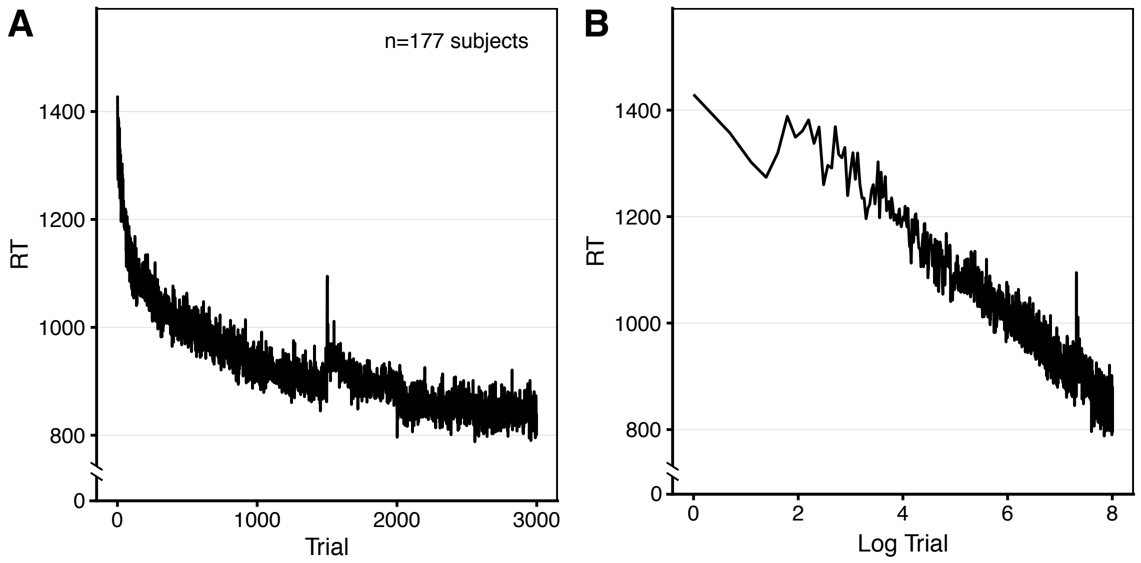


**Supplementary Figure 9.** **Log and Linear Trial Fits.** To best account for the impact of trial on reaction time (RT) in subsequent models, we plot mean RT *versus* trial across both stages of Experiments 1 and 3, for a total of 3000 trials. *(A)* Plot of Trial *versus* RT. We observe a nonlinear relationship, with an initial sharp decrease in reaction time followed by a long tail of slow improvement. *(B)* Plot of log(Trial) versus mean RT. In this semi-log space, the mean relationship appears linear. We apply this transformation in all of our subsequent models.

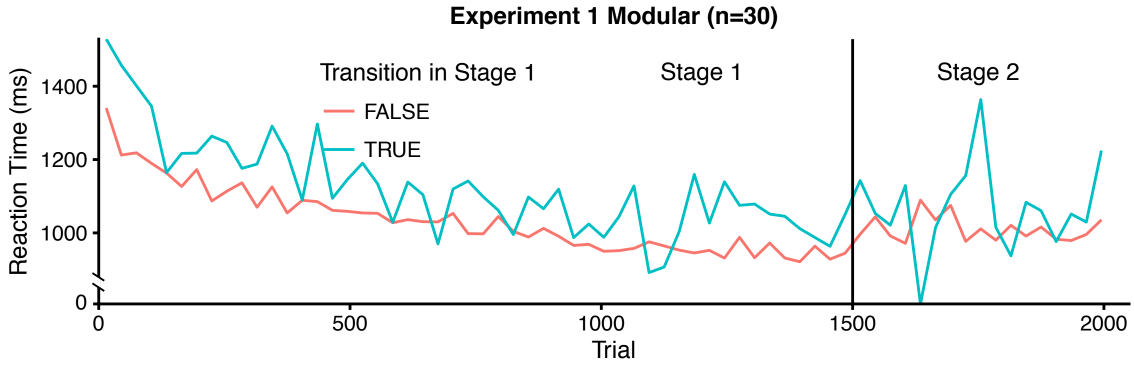


**Supplementary Figure 10.** **Surprisal Effect Maintained Across Changes in the Underlying Graph.** Mean RT across 30-trial bins after first separating the trials according to whether they were transition edges *versus* non-transition edges in stage 1 of experiment 1. We ignored all trials on edges that were not present in stage 1; thus, the data that we consider in stage 2 constitutes previously seen edges differentiated by the function that the edge served in stage 1. We observe a clear RT increase for transition edges in stage 1, as well as a smaller RT increase for transition edges in stage 2. See text for statistical testing of this effect.

## 3 Supplementary Tables

Here we report the fixed effects from methods used throughout the paper (see Methods).

| Experiment | Stage | Graph | Walk Type | Trials |
|---|---|---|---|---|
| 1 | 1 | Random/Lattice/Modular | Random | 1500 |
| | 2 | Fully Connected | Random | 500 |
| 2 | 1 | Modular | Random | 1500 |
| | 2 | Modular | Hamiltonian | 500 |
| 3 | 1 | Random/Lattice/Modular | Random | 1500 |
| | 2 | Random/Lattice/Modular | Random | 1500 |

**Supplementary Table 1. Summary of Experimental Design.** We ran three separate experiments, which varied in the underlying graph structure being traversed and in the type of traversal. Graphs were either a modular, lattice, or random structure of 15 nodes and 30 edges, or a fully connected graph of 15 nodes. Traversals were either a random walk or a Hamiltonian walk.

| | Estimate | Std. Error | 95% Conf. Int. | | df | t value | Pr(> \|t\|) | Sig. |
|---|---|---|---|---|---|---|---|---|
| (Intercept) | 1037.87 | 43.76 | 952.10 | 1123.63 | 29 | 23.72 | <0.001 | *** |
| Trial | -183.92 | 24.13 | -231.21 | -136.63 | 29 | -7.62 | <0.001 | *** |
| Transition | 63.58 | 17.61 | 29.07 | 98.10 | 29 | 3.61 | 0.0011 | ** |
| Trial:Transition | -12.54 | 21.61 | -54.91 | 29.82 | 30 | -0.58 | 0.57 | |

**Supplementary Table 2. Cross-Cluster Surprisal Effect.** To quantify RT difference for the cross-cluster surprisal effect, we fit a mixed effects model to stage 1 modular graph data from Experiment 1, and modeled RT based on Trial Number (1-1500) and Transition (True or False, whether a trial transitioned into a new cluster). Here we report fixed effects from the model. We found the effect of transition to be highly significant. Significance codes: $p$-values equal 0 '***' 0.001 '**' 0.01 '*' 0.05 '.' 0.1 ' ' 1.

| Random Walk | Estimate | Std. Error | 95% Conf. Int. | | df | t value | Pr(> \|t\|) | Sig. |
|---|---|---|---|---|---|---|---|---|
| (Intercept) | 961.96 | 32.58 | 898.10 | 1025.82 | 58 | 29.53 | <0.001 | *** |
| Trial | -191.42 | 15.11 | -221.04 | -161.80 | 58 | -12.67 | <0.001 | *** |
| Transition | 27.90 | 13.44 | 1.56 | 54.24 | 58 | 2.08 | 0.042 | * |
| Trial:Transition | 34.73 | 14.71 | 5.89 | 63.57 | 55 | 2.36 | 0.022 | * |
| **Hamiltonian Walk** | **Estimate** | **Std. Error** | **95% Conf. Int.** | | **df** | **t value** | **Pr(> \|t\|)** | **Sig.** |
| (Intercept) | 868.72 | 30.08 | 809.75 | 927.68 | 58 | 28.88 | <0.001 | *** |
| Trial | -37.67 | 8.08 | -53.51 | -21.83 | 58 | -4.66 | <0.001 | *** |
| Transition | 7.16 | 10.37 | -13.17 | 27.49 | 58 | 0.69 | 0.49 | |
| Trial:Transition | 5.52 | 13.71 | -21.35 | 32.39 | 57 | 0.40 | 0.69 | |

**Supplementary Table 3. Surprisal Effect Transfer.** To test persistence of a surprisal effect when the walk type was changed, we fit a mixed effects model separately to stages 1 and 2 of Experiment 2, where subjects first saw a 1500-trial random walk on the modular graph, followed by a 500-trial Hamiltonian walk on the same graph. Here we report fixed effects from the model. We find a significant surprisal effect for the data in the first stage but not in the second stage. Significance codes: $p$-values equal 0 '***' 0.001 '**' 0.01 '*' 0.05 '.' 0.1 ' ' 1.

| | Estimate | Std. Error | 95% Conf. Int. | | df | t value | Pr(> \|t\|) | Sig. |
|---|---|---|---|---|---|---|---|---|
| (Intercept) | 965.26 | 21.59 | 922.94 | 1007.58 | 106 | 44.70 | <0.001 | *** |
| Trial | -58.85 | 6.27 | -71.14 | -46.56 | 107 | -9.39 | <0.001 | *** |
| Graph2 (Random) | 34.80 | 50.38 | -63.94 | 133.54 | 106 | 0.69 | 0.49 | |
| Graph3 (Modular) | 100.30 | 53.05 | -3.68 | 204.28 | 106 | 1.89 | 0.061 | . |
| LearnedEdge | -25.50 | 5.86 | -37.00 | -14.01 | 131 | -4.35 | <0.001 | *** |
| Trial:Graph2 (Random) | 10.02 | 14.62 | -18.63 | 38.67 | 107 | 0.69 | 0.49 | |
| Trial:Graph3 (Modular) | 31.15 | 15.40 | 0.97 | 61.33 | 107 | 2.02 | 0.046 | * |
| Trial:LearnedEdge | 28.37 | 6.96 | 14.73 | 42.02 | 1142 | 4.08 | <0.001 | *** |
| Graph2 (Random):LearnedEdge | -4.70 | 13.76 | -31.67 | 22.27 | 134 | -0.34 | 0.73 | |
| Graph3 (Modular):LearnedEdge | 12.68 | 14.40 | -15.55 | 40.90 | 130 | 0.88 | 0.38 | |
| Trial:Graph2 (Random):LearnedEdge | 2.12 | 16.39 | -30.01 | 34.25 | 1181 | 0.13 | 0.9 | |
| Trial:Graph3 (Modular):LearnedEdge | 4.11 | 17.07 | -29.35 | 37.58 | 1134 | 0.24 | 0.81 | |

**Supplementary Table 4. Novel Edge Effect.** To estimate the change in performance when encountering a novel edge, we fit a mixed effects model to all Experiment 1 stage 2 data, when subjects were exposed to a fully connected graph. We modeled RT based on Trial Number (1-1500), LearnedEdge (True or False, whether the edge was present in stage 1), and stage 1 Graph Type (lattice, random, or modular). We find that learners show a significant increase in RT on novel edges. Significance codes: $p$-values equal 0 '***' 0.001 '**' 0.01 '*' 0.05 '.' 0.1 ' ' 1.

| Lattice vs. Random | Estimate | Std. Error | 95% Conf. Int. | | df | t value | Pr(> \|t\|) | Sig. |
|---|---|---|---|---|---|---|---|---|
| (Intercept) | 928.42 | 23.31 | 882.74 | 974.10 | 68 | 39.83 | <0.001 | *** |
| Trial | -105.20 | 7.40 | -119.70 | -90.70 | 68 | -14.22 | <0.001 | *** |
| Graph | -12.85 | 8.69 | -29.88 | 4.17 | 68 | 1.48 | 0.14 | |
| Stage | -124.33 | 8.69 | -141.35 | -107.31 | 68 | -14.32 | <0.001 | *** |
| Trial:Graph | 8.22 | 10.74 | -12.83 | 29.27 | 68 | 0.77 | 0.45 | |
| Trial:Stage | 136.73 | 10.74 | 115.68 | 157.78 | 68 | 12.73 | <0.001 | *** |
| Graph:Stage | -118.06 | 93.23 | -300.80 | 64.67 | 68 | -1.27 | 0.21 | |
| Trial:Graph:Stage | 2.87 | 29.59 | -55.12 | 60.85 | 68 | 0.10 | 0.92 | |
| **Modular vs. Lattice** | **Estimate** | **Std. Error** | **95% Conf. Int.** | | **df** | **t value** | **Pr(> \|t\|)** | **Sig.** |
| (Intercept) | 909.21 | 28.25 | 853.85 | 964.58 | 70 | 32.19 | <0.001 | *** |
| Trial | -107.82 | 6.90 | -121.34 | -94.31 | 70 | -15.64 | <0.001 | *** |
| Graph | -24.26 | 10.32 | -44.49 | -4.02 | 70 | 2.35 | 0.022 | * |
| Stage | -119.78 | 10.32 | -140.01 | -99.54 | 70 | -11.60 | <0.001 | *** |
| Trial:Graph | -1.70 | 10.90 | -23.07 | 19.66 | 70 | -0.16 | 0.88 | |
| Trial:Stage | 136.67 | 10.90 | 115.31 | 158.04 | 70 | 12.54 | <0.001 | *** |
| Graph:Stage | -315.25 | 112.99 | -536.71 | -93.78 | 70 | -2.79 | 0.0068 | ** |
| Trial:Graph:Stage | 5.75 | 27.58 | -48.31 | 59.80 | 70 | 0.21 | 0.84 | |
| **Modular vs. Random** | **Estimate** | **Std. Error** | **95% Conf. Int.** | | **df** | **t value** | **Pr(> \|t\|)** | **Sig.** |
| (Intercept) | 928.62 | 26.87 | 875.96 | 981.28 | 69 | 34.56 | <0.001 | *** |
| Trial | -111.83 | 7.21 | -125.97 | -97.70 | 69 | -15.51 | <0.001 | *** |
| Graph | -34.89 | 10.17 | -54.82 | -14.95 | 69 | 3.43 | 0.001 | ** |
| Stage | -125.19 | 10.17 | -145.13 | -105.26 | 69 | -12.31 | <0.001 | *** |
| Trial:Graph | 4.03 | 13.55 | -22.53 | 30.59 | 69 | 0.30 | 0.77 | |
| Trial:Stage | 160.20 | 13.55 | 133.64 | 186.76 | 69 | 11.82 | <0.001 | *** |
| Graph:Stage | -87.05 | 107.48 | -297.70 | 123.61 | 69 | -0.81 | 0.42 | |
| Trial:Graph:Stage | -45.35 | 28.85 | -101.90 | 11.19 | 69 | -1.57 | 0.12 | |

**Supplementary Table 5. Graph Difference Fixed Effects.** We fit a mixed effects model to the second experiment, and modeled RT based on trial number (1-1500), experiment stage (1 or 2), and graph type (lattice/random/modular). Here we report fixed effects from the model. We find a significant effect of graph type for the modular/lattice comparison as well as for the modular/random comparison on performance. We found no significant differences between lattice and random graphs (see main manuscript). Significance codes: $p$-values equal 0 '***' 0.001 '**' 0.01 '*' 0.05 '.' 0.1 ' ' 1.

| | Estimate | Std. Error | 95% Conf. Int. | | df | t value | Pr(> \|t\|) | Sig. |
|---|---|---|---|---|---|---|---|---|
| (Intercept) | 1089.21 | 51.19 | 988.87 | 1189.55 | 29 | 21.28 | <0.001 | *** |
| Trial (scaled 0 to 1) | -74.20 | 21.42 | -116.18 | -32.22 | 30 | -3.46 | 0.0016 | ** |
| Transition in 1 | 113.71 | 54.23 | 7.43 | 219.99 | 30 | 2.10 | 0.045 | * |
| Edge In 1 | -67.05 | 18.67 | -103.65 | -30.46 | 34 | -3.59 | 0.001 | ** |
| Trial:Transition in 1 | -109.48 | 70.31 | -247.30 | 28.33 | 50 | -1.56 | 0.13 | |
| Trial:Edge In 1 | 49.33 | 26.33 | -2.27 | 100.93 | 57 | 1.87 | 0.066 | . |

**Supplementary Table 6. Surprisal Effect After a Change in the Graph Model.** We fit a mixed effects model to stage 2 of Experiment 1, where subjects first saw a 1500-trial random walk on the modular graph, followed by a 500-trial random walk on a fully connected graph. Here we report fixed effects from the model. We find a significant increase in RT when an edge had served as a transition in the first stage. Significance codes: p-values equal 0 '***' 0.001 '**' 0.01 '*' 0.05 '.' 0.1 ' ' 1.
